# Supplementary material for: Interplay between magnetism and short-range order in medium- and high-entropy alloys: CrCoNi, CrFeCoNi, and CrMnFeCoNi
Source: arXiv:2303.00641 ancillary file (2023-04-18)
Supplement: Supplementary file 1 [file supplemental.pdf]

# Interplay between magnetism and short-range order in medium- and high-entropy alloys: CrCoNi, CrFeCoNi, and CrMnFeCoNi

Christopher D. Woodgate,[1] Daniel Hedlund,[2] L. H. Lewis,[2,3] and Julie B. Staunton[1]

[1]*Department of Physics, University of Warwick, Coventry, CV4 7AL, United Kingdom*

[2]*Department of Chemical Engineering, Northeastern University, Boston, MA 02115, USA*

[3]*Department of Mechanical and Industrial Engineering, Northeastern University, Boston, MA 02115, USA*

This is the supplemental material accompanying the main text. Tables I, II, and III give the fitted atom-atom interchange parameters for the pairwise Bragg-Williams Hamiltonian for CrCoNi, CrFeCoNi, and CrMnFeCoNi respectively, for both paramagnetic and magnetically ordered states. The Hamiltonian is

$$H = \frac{1}{2} \sum_{i\alpha;j\alpha'} V_{i\alpha;j\alpha'} \xi_{i\alpha} \xi_{j\alpha'} + \sum_{i\alpha} \nu_\alpha \xi_{i\alpha}, \tag{1}$$

where we drop the term involving the chemical potential as our simulations use Kawasaki dynamics to conserve overall concentration of each species. We assume $V_{i\alpha;j\alpha'}$ are homogeneous and isotropic and write $V^{(n)}_{\alpha\alpha'}$ to denote the interaction between species $\alpha$ and $\alpha'$ on coordination shell $n$. We sample 56 **k**-points around the irreducible Brillouin zone, including high-symmetry directions, to fit an interaction to the first four coordination shells, to enable comparison with the results shown in Ref. [1]. The formal definition of $V_{i\alpha;j\alpha'}$ and the convention used to fix the gauge degree of freedom can be found in Ref. [2]. Some discussion of the fitting procedure can also be found in Ref. [3].

[1] C. D. Woodgate and J. B. Staunton, Physical Review B **105**, 115124 (2022).

[2] S. N. Khan, J. B. Staunton, and G. M. Stocks, Phys. Rev. B **93**, 054206 (2016).

[3] C. D. Woodgate and J. B. Staunton, Physical Review Materials **7**, 013801 (2023).

| Paramagnetic | | | | Magnetically Ordered | | | |
|---|---|---|---|---|---|---|---|
| $V^{(1)}_{\alpha\alpha'}$ | Ni | Co | Cr | $V^{(1)}_{\alpha\alpha'}$ | Ni | Co | Cr |
| Ni | −0.218 | 0.682 | −0.465 | Ni | −0.147 | 0.461 | −0.315 |
| Co | 0.682 | 0.673 | −1.351 | Co | 0.461 | 0.247 | −0.704 |
| Cr | −0.465 | −1.351 | 1.813 | Cr | −0.315 | −0.704 | 1.017 |
| $V^{(2)}_{\alpha\alpha'}$ | Ni | Co | Cr | $V^{(2)}_{\alpha\alpha'}$ | Ni | Co | Cr |
| Ni | 0.266 | 0.032 | −0.296 | Ni | 0.273 | 0.022 | −0.293 |
| Co | 0.032 | 0.004 | −0.035 | Co | 0.022 | 0.003 | −0.025 |
| Cr | −0.296 | −0.035 | 0.330 | Cr | −0.293 | −0.025 | 0.316 |
| $V^{(3)}_{\alpha\alpha'}$ | Ni | Co | Cr | $V^{(3)}_{\alpha\alpha'}$ | Ni | Co | Cr |
| Ni | 0.021 | 0.099 | −0.120 | Ni | 0.024 | 0.056 | −0.080 |
| Co | 0.099 | 0.052 | −0.151 | Co | 0.056 | 0.015 | −0.070 |
| Cr | −0.120 | −0.151 | 0.270 | Cr | −0.080 | −0.070 | 0.150 |
| $V^{(4)}_{\alpha\alpha'}$ | Ni | Co | Cr | $V^{(4)}_{\alpha\alpha'}$ | Ni | Co | Cr |
| Ni | 0.239 | −0.005 | −0.232 | Ni | 0.208 | −0.001 | −0.206 |
| Co | −0.005 | −0.050 | 0.056 | Co | −0.001 | 0.025 | −0.024 |
| Cr | −0.232 | 0.056 | 0.175 | Cr | −0.206 | −0.024 | 0.229 |

TABLE I: Interchange parameters for CrCoNi at the specified equiatomic composition fitted from $S^{(2)}_{\alpha\alpha'}(\mathbf{k})$ evaluated at $T = 1000K$, in units of mRy.

| Paramagnetic | | | | | Magnetically Ordered | | | | |
|---|---|---|---|---|---|---|---|---|---|
| $V^{(1)}_{\alpha\alpha'}$ | Ni | Co | Fe | Cr | $V^{(1)}_{\alpha\alpha'}$ | Ni | Co | Fe | Cr |
| Ni | −0.338 | 0.607 | 0.097 | −0.366 | Ni | −0.030 | 0.359 | −0.139 | −0.189 |
| Co | 0.607 | 0.655 | −0.049 | −1.213 | Co | 0.359 | 0.240 | −0.032 | −0.567 |
| Fe | 0.097 | −0.049 | −0.019 | −0.029 | Fe | −0.139 | −0.032 | 0.631 | −0.459 |
| Cr | −0.366 | −1.213 | −0.029 | 1.609 | Cr | −0.189 | −0.567 | −0.459 | 1.216 |
| $V^{(2)}_{\alpha\alpha'}$ | Ni | Co | Fe | Cr | $V^{(2)}_{\alpha\alpha'}$ | Ni | Co | Fe | Cr |
| Ni | 0.316 | 0.058 | −0.061 | −0.313 | Ni | 0.285 | 0.035 | −0.038 | −0.282 |
| Co | 0.058 | 0.005 | −0.007 | −0.057 | Co | 0.035 | 0.013 | −0.090 | 0.041 |
| Fe | −0.061 | −0.007 | 0.010 | 0.058 | Fe | −0.038 | −0.090 | −0.159 | 0.287 |
| Cr | −0.313 | −0.057 | 0.058 | 0.312 | Cr | −0.282 | 0.041 | 0.287 | −0.046 |
| $V^{(3)}_{\alpha\alpha'}$ | Ni | Co | Fe | Cr | $V^{(3)}_{\alpha\alpha'}$ | Ni | Co | Fe | Cr |
| Ni | 0.002 | 0.090 | 0.008 | −0.100 | Ni | 0.014 | 0.027 | −0.042 | 0.002 |
| Co | 0.090 | 0.053 | −0.009 | −0.135 | Co | 0.027 | 0.007 | 0.009 | −0.042 |
| Fe | 0.008 | −0.009 | −0.002 | 0.003 | Fe | −0.042 | 0.009 | 0.110 | −0.076 |
| Cr | −0.100 | −0.135 | 0.003 | 0.232 | Cr | 0.002 | −0.042 | −0.076 | 0.117 |
| $V^{(4)}_{\alpha\alpha'}$ | Ni | Co | Fe | Cr | $V^{(4)}_{\alpha\alpha'}$ | Ni | Co | Fe | Cr |
| Ni | 0.255 | 0.006 | −0.032 | −0.229 | Ni | 0.144 | 0.015 | 0.076 | −0.236 |
| Co | 0.006 | −0.046 | −0.001 | 0.041 | Co | 0.015 | 0.036 | 0.050 | −0.101 |
| Fe | −0.032 | −0.001 | 0.004 | 0.030 | Fe | 0.076 | 0.050 | −0.058 | −0.068 |
| Cr | −0.229 | 0.041 | 0.030 | 0.158 | Cr | −0.236 | −0.101 | −0.068 | 0.405 |

TABLE II: Interchange parameters for CrFeCoNi at the specified equiatomic composition fitted from $S^{(2)}_{\alpha\alpha'}(\mathbf{k})$ evaluated at $T = 1000K$, in units of mRy.

| Paramagnetic | | | | | | Magnetically Ordered | | | | | |
|---|---|---|---|---|---|---|---|---|---|---|---|
| $V^{(1)}_{\alpha\alpha'}$ | Ni | Co | Fe | Mn | Cr | $V^{(1)}_{\alpha\alpha'}$ | Ni | Co | Fe | Mn | Cr |
| Ni | −0.464 | 0.528 | 0.097 | 0.183 | −0.344 | Ni | −0.386 | 0.318 | −0.115 | 0.410 | −0.227 |
| Co | 0.528 | 0.701 | 0.063 | −0.282 | −1.010 | Co | 0.318 | 0.330 | −0.073 | −0.037 | −0.538 |
| Fe | 0.097 | 0.063 | 0.002 | −0.048 | −0.114 | Fe | −0.115 | −0.073 | 0.461 | −0.438 | 0.165 |
| Mn | 0.183 | −0.282 | −0.048 | −0.067 | 0.214 | Mn | 0.410 | −0.037 | −0.438 | 0.222 | −0.156 |
| Cr | −0.344 | −1.010 | −0.114 | 0.214 | 1.253 | Cr | −0.227 | −0.538 | 0.165 | −0.156 | 0.757 |
| $V^{(2)}_{\alpha\alpha'}$ | Ni | Co | Fe | Mn | Cr | $V^{(2)}_{\alpha\alpha'}$ | Ni | Co | Fe | Mn | Cr |
| Ni | 0.435 | 0.129 | −0.016 | −0.229 | −0.319 | Ni | 0.455 | 0.129 | −0.005 | −0.255 | −0.324 |
| Co | 0.129 | 0.036 | 0.001 | −0.070 | −0.096 | Co | 0.129 | 0.054 | −0.067 | −0.003 | −0.113 |
| Fe | −0.016 | 0.001 | −0.000 | 0.008 | 0.008 | Fe | −0.005 | −0.067 | −0.256 | 0.258 | 0.070 |
| Mn | −0.229 | −0.070 | 0.008 | 0.121 | 0.171 | Mn | −0.255 | −0.003 | 0.258 | −0.114 | 0.113 |
| Cr | −0.319 | −0.096 | 0.008 | 0.171 | 0.235 | Cr | −0.324 | −0.113 | 0.070 | 0.113 | 0.254 |
| $V^{(3)}_{\alpha\alpha'}$ | Ni | Co | Fe | Mn | Cr | $V^{(3)}_{\alpha\alpha'}$ | Ni | Co | Fe | Mn | Cr |
| Ni | 0.007 | 0.092 | 0.014 | −0.009 | −0.104 | Ni | 0.010 | 0.052 | −0.012 | 0.021 | −0.071 |
| Co | 0.092 | 0.062 | 0.006 | −0.047 | −0.112 | Co | 0.052 | 0.037 | 0.035 | −0.057 | −0.067 |
| Fe | 0.014 | 0.006 | 0.000 | −0.007 | −0.013 | Fe | −0.012 | 0.035 | 0.130 | −0.125 | −0.028 |
| Mn | −0.009 | −0.047 | −0.007 | 0.007 | 0.056 | Mn | 0.021 | −0.057 | −0.125 | 0.108 | 0.052 |
| Cr | −0.104 | −0.112 | −0.013 | 0.056 | 0.173 | Cr | −0.071 | −0.067 | −0.028 | 0.052 | 0.115 |
| $V^{(4)}_{\alpha\alpha'}$ | Ni | Co | Fe | Mn | Cr | $V^{(4)}_{\alpha\alpha'}$ | Ni | Co | Fe | Mn | Cr |
| Ni | 0.296 | 0.027 | −0.003 | −0.138 | −0.182 | Ni | 0.270 | 0.045 | 0.058 | −0.197 | −0.177 |
| Co | 0.027 | −0.040 | −0.002 | −0.010 | 0.025 | Co | 0.045 | 0.026 | 0.053 | −0.075 | −0.050 |
| Fe | −0.003 | −0.002 | −0.000 | 0.001 | 0.004 | Fe | 0.058 | 0.053 | −0.056 | 0.032 | −0.087 |
| Mn | −0.138 | −0.010 | 0.001 | 0.064 | 0.083 | Mn | −0.197 | −0.075 | 0.032 | 0.062 | 0.177 |
| Cr | −0.182 | 0.025 | 0.004 | 0.083 | 0.070 | Cr | −0.177 | −0.050 | −0.087 | 0.177 | 0.137 |

TABLE III: Interchange parameters for CrMnFeCoNi at the specified equiatomic composition fitted from $S^{(2)}_{\alpha\alpha'}(\mathbf{k})$ evaluated at $T = 1000K$, in units of mRy.
